# Supplementary material for: Tuning colloid-interface interactions by salt partitioning
Source: arXiv:1603.08703 ancillary file (2016-08-24)
Supplement: Supplementary file 1 [file supplementary.pdf]

# Supplemental Information: Tuning colloid-interface interactions by salt partitioning

J. C. Everts, S. Samin, and R. van Roij
*Institute for Theoretical Physics, Center for Extreme Matter and Emergent Phenomena,*
*Utrecht University, Leuvenlaan 4, 3584 CE Utrecht, The Netherlands*
(Dated: August 24, 2016)

## I. NON-TOUCHING BEHAVIOUR OF CHARGED POLY(METHYLMETHACRYLATE) (PMMA) PARTICLES NEAR AN OIL-WATER INTERFACE

In this section (Fig. S1) we show some illustrative microscope images of non-touching PMMA particles near a water-cyclohexylbromide (CHB) interface. Because of practical reasons the images are taken for a water-in-oil Pickering emulsion and not in the two-dimensional setup that we consider in the main text, see for more details Ref. [S1].

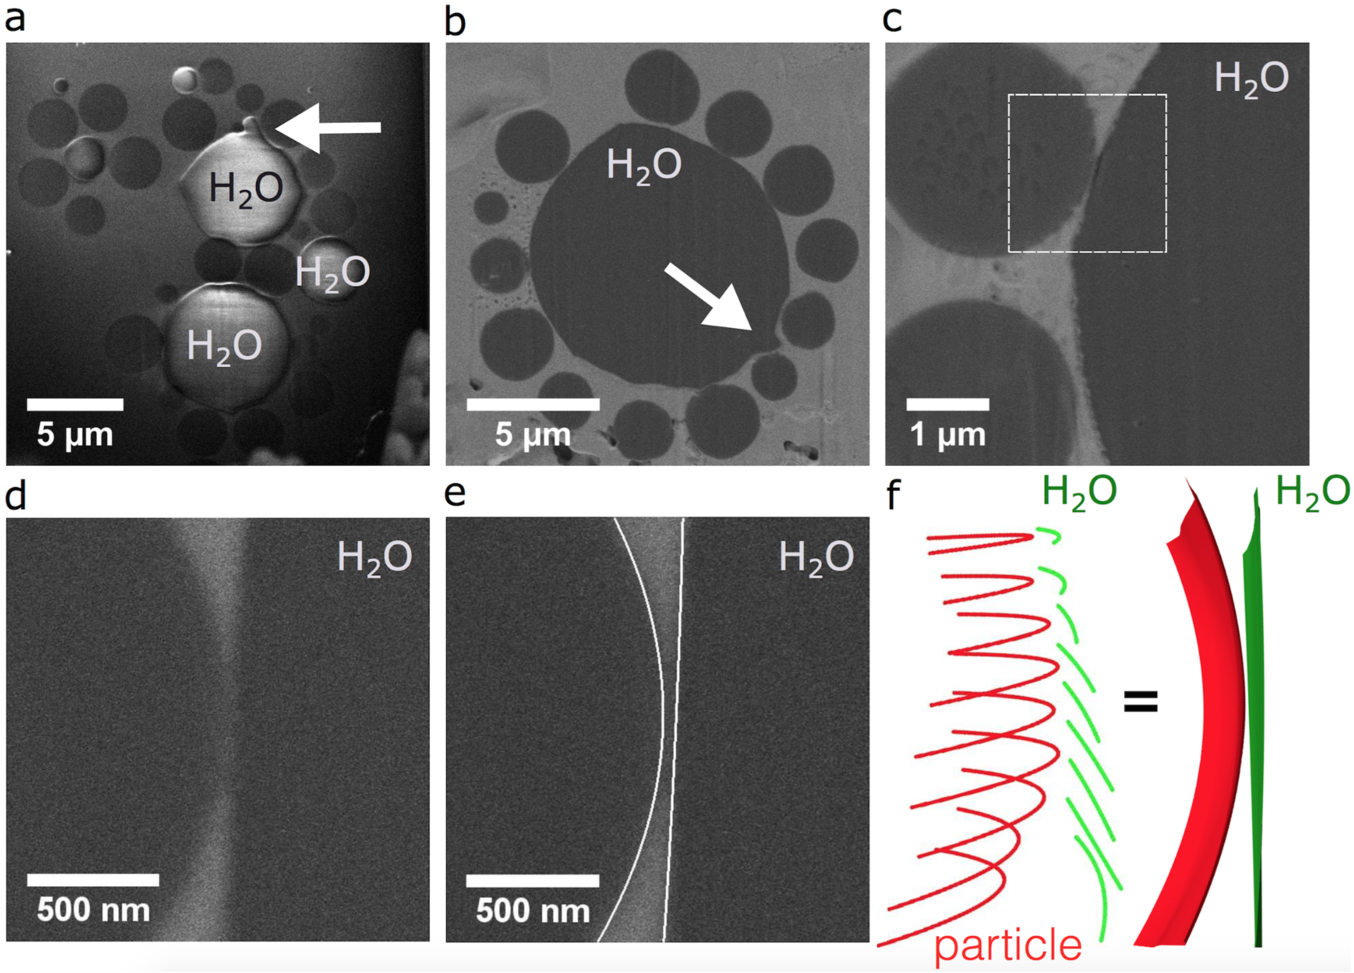


Figure S1. (Color online) Cryo - Focused Ion Beam - Scanning Electron Microscopy (Cryo-FIB-SEM) images and 3D reconstructions of the non-touching PMMA colloidal particles at a CHB-water interface. (a) A FIB milled cross section through water droplets covered with non-touching PMMA colloidal particles. Water droplets charged up in secondary electron imaging mode, allowing direct discrimination between the droplets and the PMMA particles. ((b),(c)) No breaching of the oil-water interface by the PMMA particles was observed, images recorded in back scattering mode. ((d)-(f)) FIB-SEM tomography series were used to image the intervening oil layer between the PMMA particles and the interface. Images are close-ups of the regions indicated with the white squares in (c). Surfaces were located using a polynomial function (e), and resulted in the 3D reconstructions shown in (f). Reproduced from Ref. [S1] with permission from authors and the Royal Society of Chemistry.

## II. SALT-INDUCED DISLODGEMENT OF CHARGED PMMA PARTICLES FROM AN OIL-WATER INTERFACE

In this section we show some illustrative microscope images of non-touching PMMA particles dislodging from a water-cyclohexylbromide (CHB) interface by the addition of the organic salt tetrabutylammoniumbromide to CHB (Fig. S2). See for more details Ref. [S1].

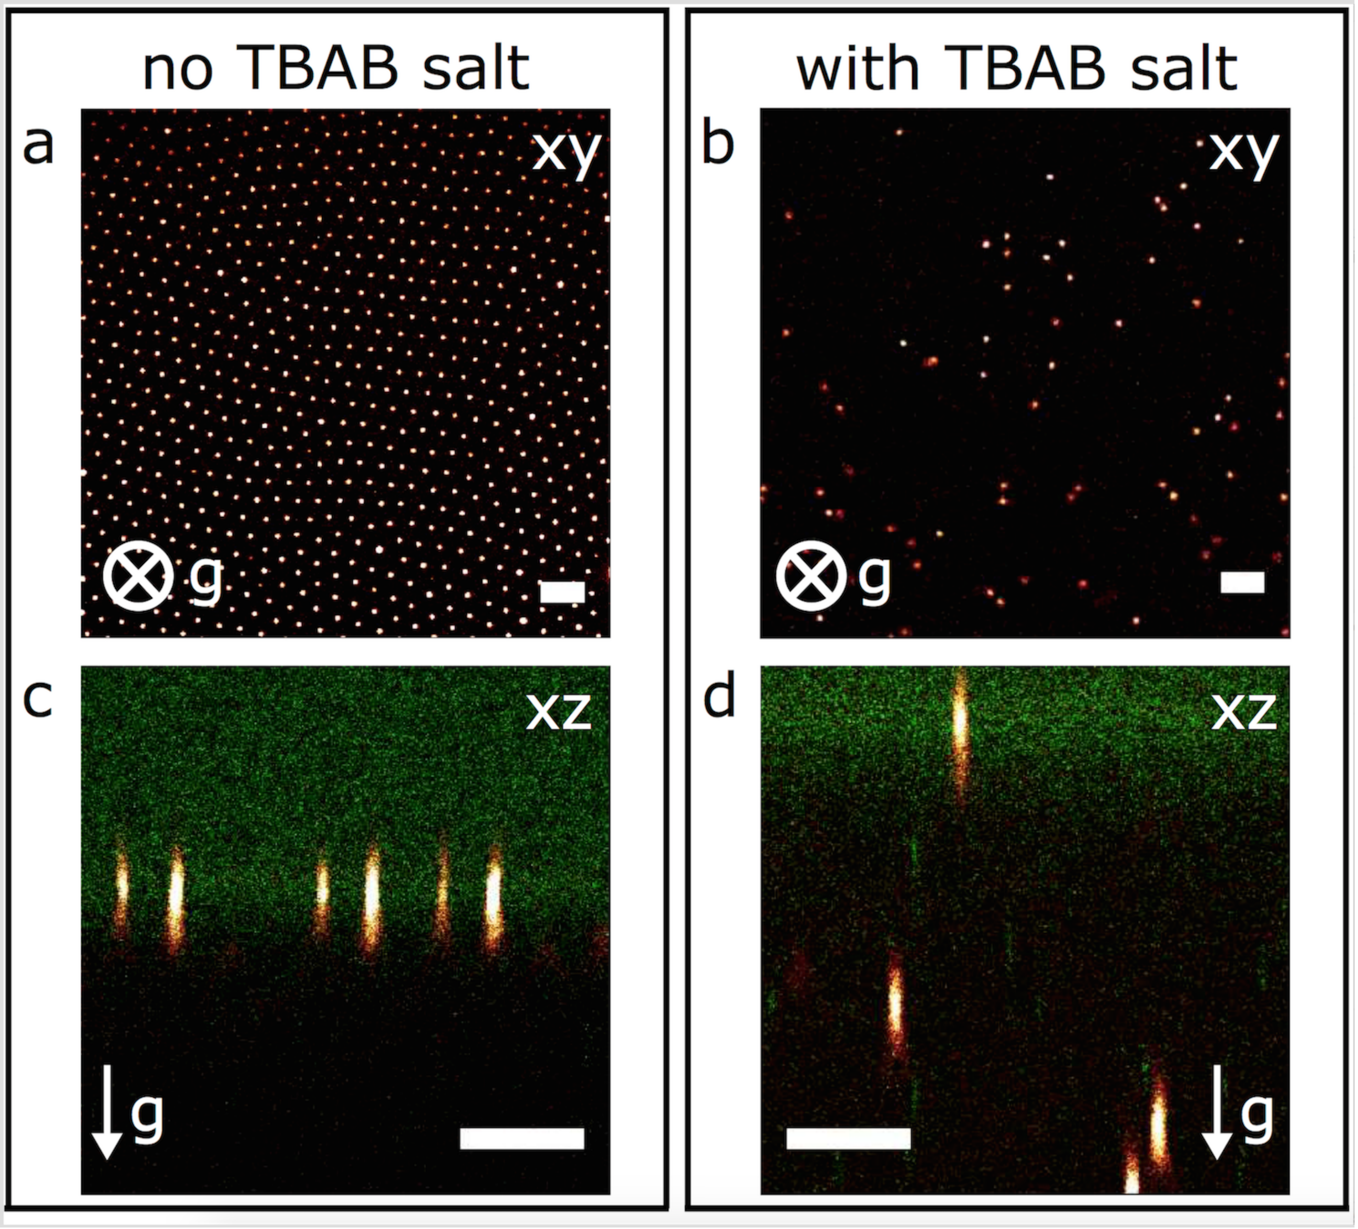


Figure S2. (Color online) Salt-induced particle dislodgement of non-touching PMMA particles from an oil-water interface. ((a)-(d)), Confocal micrographs recorded in a 2D-setup, before ((a),(c)) and directly after (t∼5 min) ((b),(d)) adding 150 $\mu$M tetrabutylammoniumbromide salt to the oil (CHB) phase. The water phase (depicted in green) was fluorescently labeled with fluorescein isothiocyanate. The interfacial structure of the PMMA colloids (depicted in glow) was imaged in the $xy$-direction ((a),(b)), the particle dislodgement from the interface was imaged in the $xz$-direction ((c),(d)). Scale bars indicate 25 $\mu$m. Reproduced from Ref. [S1] with permission from the authors and the Royal Society of Chemistry.

.

## III. EFFECT OF A REPULSIVE VAN DER WAALS INTERACTION ON THE COLLOID-INTERFACE EFFECTIVE POTENTIAL

The van der Waals interaction for a sphere of radius $a$ at a distance $d$ from a planar interface is given by [S2]

$$\Phi_{\mathrm{VdW}}(d) = -\frac{A_H}{6}\left[\frac{1}{d/a-1} + \frac{1}{d/a+1} + \ln\left(\frac{d/a-1}{d/a+1}\right)\right], \tag{S.1}$$

which reduces to $\Phi_{\mathrm{VdW}}(d) = -A_H/[6(d/a-1)]$ for $d/a-1 \ll 1$, with $A_H$ the Hamaker constant. We now investigate how $\Phi_{\mathrm{VdW}}(d)$ would act on top of the electrostatic interactions given by $\Phi(d) = H(d) - H(\infty)$, with

$$\begin{aligned}\beta H(d) = &-\frac{1}{2}\int_\Gamma d^2\mathbf{r}\;\sigma(\mathbf{r})\phi(\mathbf{r}) + \int_{\mathcal{R}} d^3\mathbf{r}\;\rho_s(z)\Big\{\phi(\mathbf{r})\sinh[\phi(\mathbf{r})-\Theta(z)\phi_D] - 2(\cosh[\phi(\mathbf{r})-\Theta(z)\phi_D]-1)\Big\}\\ &-\sigma_m\int_\Gamma d^2\mathbf{r}\ln\left\{1+\frac{\rho_s^o}{K_\pm}\exp[\mp(\phi(\mathbf{r})-\phi_D)]\right\},\end{aligned} \tag{S.2}$$

see Fig. S3 . As explained in the text, we indeed see that $\Phi_{\mathrm{VdW}}$ is only important for small $d$, but it is strong enough to impede adsorption of the colloid on the oil-water interface. This also shows that the location of the minimum depends on the magnitude of the colloidal charge, which is not different from the results of Ref. [S3], since a force balance between Van der Waals repulsion and image charge attractions also give rise to a equilibrium distance that depends on $Z$. The new feature is that the sign of $Z$ and $\phi_D$ matters for the type of interaction (repulsion or attraction) when salt is included, and these are largely tunable as explained in the main text.

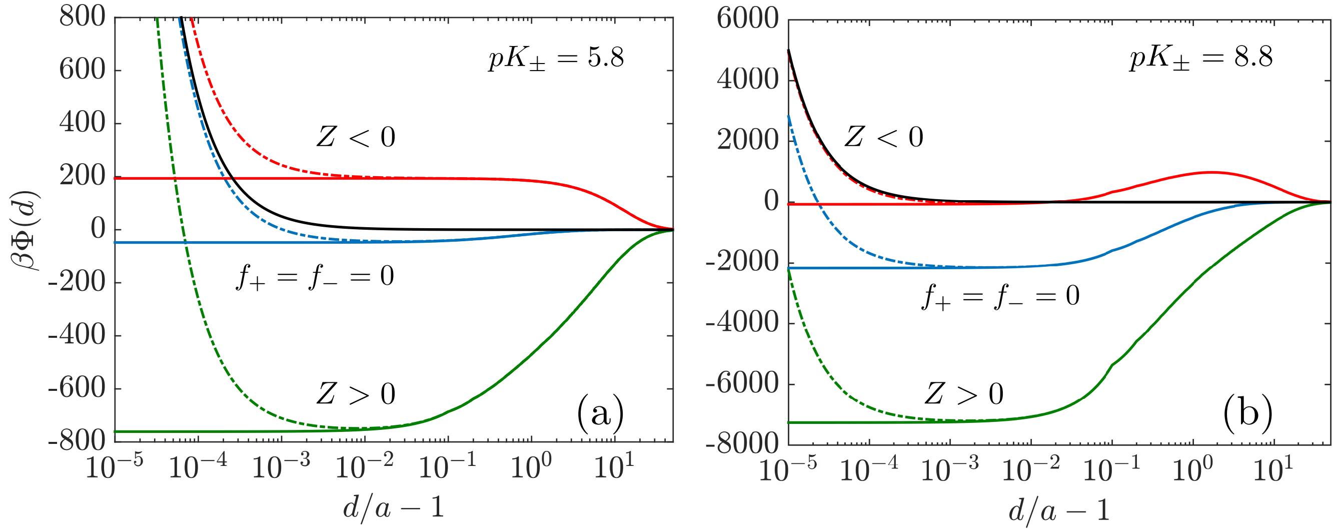


Figure S3. (Color online) Contributions to the colloid-interface potential as a function of the surface-to-surface separation $d-a$ in units of the colloidal radius $a = 1$ $\mu$m, where $d$ is the center-to-surface distance between sphere and interface. The full lines are the same colloid-interface potential $\Phi(d)$ as is plotted in Fig. 3 (main text) for the charge regulation cases. The black full line is the van der Waals interaction $\Phi_{\mathrm{VdW}}$ with Hamaker constant $\beta A_H = -0.3$ and the dashed-dotted lines show $\Phi(d) + \Phi_{\mathrm{VdW}}(d)$, showing that the Van der Waals forces give significant additional repulsion only for $d - a \lesssim 10^{-2}a = 10$ nm, but strong enough to overcome the attractions induced by the Donnan potential for $Z > 0$.

## IV. CONSTANT-CHARGE BOUNDARY CONDITIONS

In the main text, we use charge-regulation boundary condition. Instead, we could also have used constant-charge boundary conditions, with for the particle surface, we have the boundary condition $\mathbf{n}\cdot[\epsilon_c\nabla\phi|_{\rm in}-\epsilon_o\nabla\phi|_{\rm out}]/\epsilon_o = Z\lambda_B^o/a^2$, with $Z$ now a given constant. The effective Hamiltonian for constant-charge particles is given by

$$\beta H(d) = \frac{Z}{8\pi a^2}\int_\Gamma d^2\mathbf{r}\ \phi(\mathbf{r}) + \int_{\mathcal{R}} d^3\mathbf{r}\ \rho_s(z)\Big\{\phi(\mathbf{r})\sinh[\phi(\mathbf{r})-\Theta(z)\phi_D] - 2(\cosh[\phi(\mathbf{r})-\Theta(z)\phi_D]-1)\Big\}. \tag{S.3}$$

We will see that the approximation $\tilde{\Phi}(d)$ for $\Phi(d) = H(d) - H(\infty)$ as mentioned in the text is much better for constant-charge particles than it is for charge-regulating particles, see Fig. S4

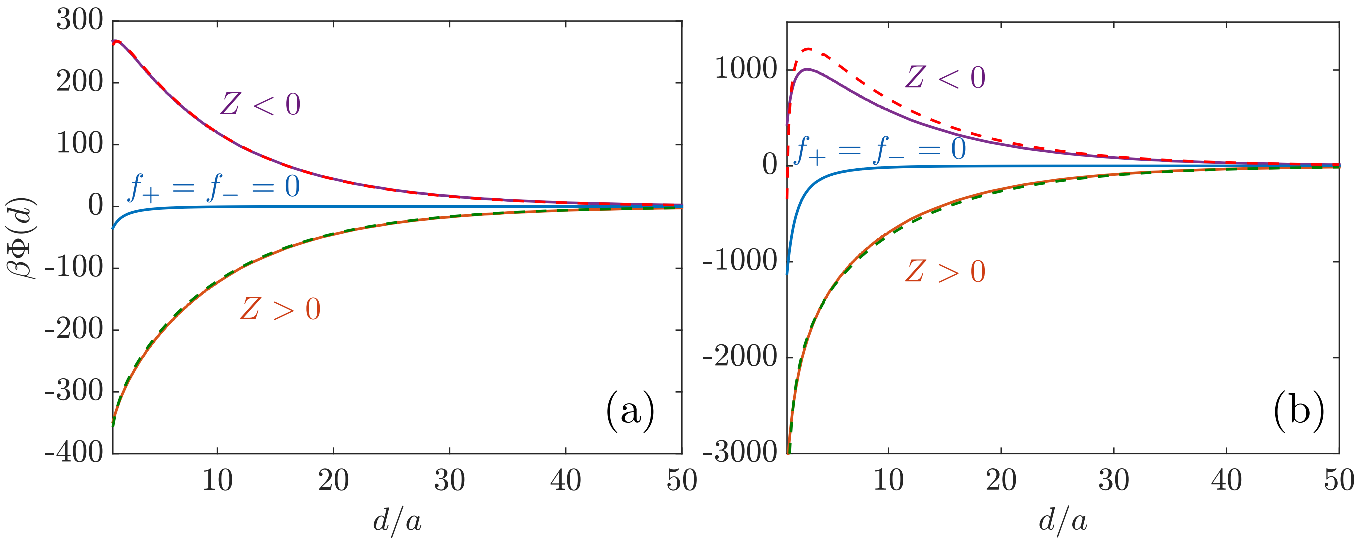


Figure S4. (Color online) Particle-interface potential $\Phi(d)$ for oil screening length $\kappa_o^{-1} = 10a$. The full curves are the results of a constant-charge boundary condition with a charge $Z$ that matches the charge at $d\to\infty$ in the case of a charge-regulation model with (a) $pK_\pm = 5.8$ and (b) $pK_\pm = 8.8$ (see Fig. 3). The purple (orange) curves are for a negative (positive) particle with self-energies $(f_+, f_-) = (6, 10)$, the blue curves are for $f_+ = f_- = 0$ and are independent of the sign of $Z$. The green ($Z > 0$) and red ($Z < 0$) dashed curves show the approximation $\tilde{\Phi}(d)$. When compared to Fig. 3 in the main text it is obvious that $\tilde{\Phi}(d)$ approximates the constant-charge case better than the charge-regulation case.


[S1] N. Elbers, J. van der Hoeven, M. de Winter, C. Schneijdenberg, M. van der Linden, L. Filion, and A. van Blaaderen, Soft Matter , (2016).

[S2] V. A. Parsegian, “Van der waals forces: A handbook for biologists, chemists, engineers, and physicists,” Cambridge Press (2005).

[S3] M. Oettel, Phys. Rev. E **76**, 041403 (2007).
